# Supplementary material for: Data-driven Nonlinear Predictive Control for Feedback Linearizable Systems
Source: arXiv:2211.06339 source file (2023-03-27)
Supplement: Supplementary file 1 [file appendix.tex]

\appendix
\section{Choice of basis functions}
\label{app_BF}
\textcolor{blue}{To approximate $\mathbf{v}_k$ in \eqref{linearizing_controller_dt}, we use the following choice of basis functions
	\begin{align*}
		\Psi(\tau_k,\Xi_k) = \,&\eta_1(\Xi_{k})\cdot\\
		&\big[ \begingroup\setlength\arraycolsep{5pt}\begin{matrix}
			\tau_{1,k} & \tau_{2,k} & \tau_{1,k}\cos(\xi_{3,k}) & \tau_{2,k}\cos(\xi_{3,k})
		\end{matrix}\endgroup\\
		&\hspace{2mm}\begingroup\setlength\arraycolsep{4pt}
		\begin{matrix}
			\cos(\xi_{1,k}) & \cos(\xi_{3,k}) & \cos(\xi_{1,k})\cos(\xi_{3,k})
		\end{matrix}
		\endgroup\\
		&\hspace{2mm}\begingroup\setlength\arraycolsep{4pt}\begin{matrix}
			\cos(\xi_{1,k}+\xi_{3,k}) & \cos(\xi_{1,k}+\xi_{3,k})\cos(\xi_{3,k})
		\end{matrix}\endgroup\\
		&\hspace{2mm}\begingroup\setlength\arraycolsep{4pt}\begin{matrix}
			\eta_2(\Xi_k)\sin(\xi_{3,k}) & \eta_2(\Xi_k)\sin(\xi_{3,k})\cos(\xi_{3,k})
		\end{matrix}\endgroup\\
		&\hspace{2mm}\begingroup\setlength\arraycolsep{4pt}\begin{matrix}
			\eta_3(\Xi_k)\sin(\xi_{3,k}) & \eta_3(\Xi_k)\sin(\xi_{3,k})\cos(\xi_{3,k})
		\end{matrix}\endgroup\\
		&\hspace{2mm}\begingroup\setlength\arraycolsep{4pt}\begin{matrix}
			\eta_4(\Xi_k)\sin(\xi_{3,k}) & \eta_4(\Xi_k)\sin(\xi_{3,k})\cos(\xi_{3,k})
		\end{matrix}\endgroup\big]^\top,
		%\label{choice_of_Psi}
	\end{align*}
	where\footnote{We use $\otimes$ to denote the Kronecker product.}
	\begin{equation*}
		\begin{aligned}
			\eta_1(\Xi_k) &= I_r\otimes(1+\cos^2(\xi_{3,k})),\\
			\eta_2(\Xi_k) &=  \left(\frac{\xi_{2,k}-\xi_{1,k}}{T_s}\right)^2,\\
			\eta_3(\Xi_k) &=  \left(\frac{\xi_{4,k}-\xi_{3,k}}{T_s}\right)^2,\\
			\eta_4(\Xi_k) &= \sqrt{\eta_2(\Xi_k)\eta_3(\Xi_k)}.
		\end{aligned}
\end{equation*}}

\textcolor{blue}{Notice that $\eta_2(\Xi_k),\eta_3(\Xi_k)$ represent the state measurements $x_{2,k},x_{4,k}$, respectively, whose structure is known due to the assumed known coordinate transformation \eqref{coordinate_transformation}.}
